# Supplementary material for: Assessing zero-shot generalisation behaviour in graph-neural-network interatomic potentials
Source: arXiv:2502.21317 ancillary file (2025-03-13)
Supplement: Supplementary file 1 [file supp_mat.pdf]

# Supplementary Information for “Assessing zero-shot generalisation behaviour in graph-neural-network interatomic potentials”

Chiheb Ben Mahmoud,<sup>1,\*</sup> Zakariya El-Machachi,<sup>1</sup> Krystian A. Gierczak,<sup>1</sup> John L. A. Gardner,<sup>1</sup> and Volker L. Deringer<sup>1</sup>

<sup>1</sup>*Inorganic Chemistry Laboratory, Department of Chemistry,  
University of Oxford, Oxford OX1 3QR, United Kingdom*

(Dated: March 13, 2025)

## I. HYPERPARAMETERS OF GRAPH-NEURAL NETWORKS TRAINED ON THE GRAPHENE OXIDE DATASET

In Table S1, we report the main hyperparameters of the GNNs trained on the GO dataset. For PaiNN, SchNet, NequIP and TensorNet (see references in the main text), we used a radial cut-off of 3.7 Å, and targeted  $\approx 150,000$  parameters. These choices were made to ensure comparable model sizes while maintaining diversity in architectural design across different GNNs. We also include the main hyperparameters of GO-MACE-23 and the MACE-OFF models used herein.

Table S1: Hyperparameters of GNNs used in this work

| MLIP          | cutoff (Å) | Layers | Channels per Layer                            | Radial Features |
|---------------|------------|--------|-----------------------------------------------|-----------------|
| GO-MACE-23    | 3.7        | 2      | 128x0e + 128x1o                               | 8               |
| MACE-OFF23(L) | 5.0        | 2      | 192x0e + 192x1o + 192x2e                      | 8               |
| MACE-OFF24    | 6.0        | 2      | 128x0e + 128x1o                               | 8               |
| PaiNN         | 3.7        | 3      | 64                                            | 16              |
| SchNet        | 3.7        | 3      | 128                                           | 64              |
| NequIP        | 3.7        | 3      | 32x0e + 32x0o + 32x1e + 32x1o + 32x2e + 32x2o | 16              |
| TensorNet     | 3.7        | 2      | 64                                            | 32              |

## II. VALIDATION ERROR OF GRAPH-NEURAL NETWORKS TRAINED ON THE GRAPHENE OXIDE DATASET

In Table S2, we report the energy and force validation RMSE of MLIP models trained on the graphene dataset.

Table S2: Validation errors on energy and forces for the different MLIPs trained on the graphene oxide dataset

| MLIP       | Energy RMSE (meV at. <sup>-1</sup> ) | Forces RMSE (eV Å <sup>-1</sup> ) |
|------------|--------------------------------------|-----------------------------------|
| GO-MACE-23 | 1.8                                  | 110                               |
| SchNet     | 6.6                                  | 361                               |
| PaiNN      | 3.0                                  | 207                               |
| TensorNet  | 2.3                                  | 182                               |
| NequIP     | 2.7                                  | 182                               |

\* chiheb.benmahmoud@chem.ox.ac.uk

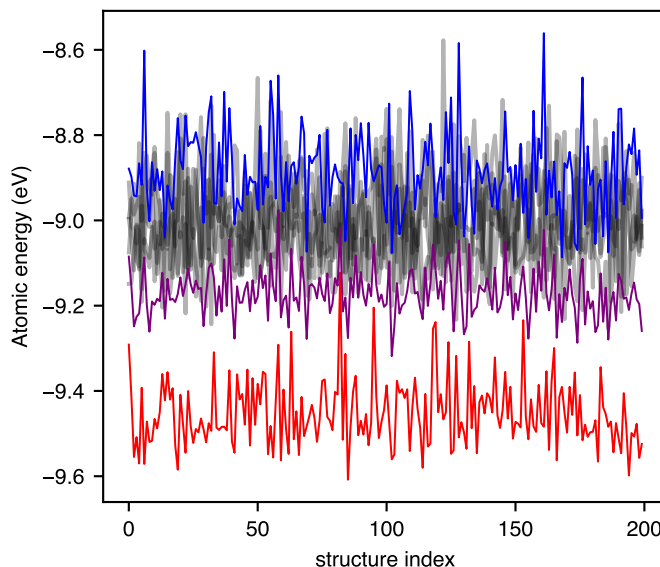

Figure S1: Atomic energies as predicted by G0-MACE-23 for 200 structures. Red, blue and purple represent the atomic energy of the carbon in the aromatic ring directly connected to the methyl group, the methyl carbon, and their average, respectively. The black curves represent the atomic energies of the remainder of the carbon atoms in the aromatic ring.

### III. ATOMIC ENERGIES OF TOLUENE

In Fig. S1, we show the local atomic energies of 200 snapshots from the toluene trajectory, as predicted by G0-MACE-23.

### IV. ENCAPSULATED MOLECULES IN $C_{60}$ CAGES

In Fig. S2, we show the evolution of energy and forces errors of three encapsulated reactions:  $H_2O@C_{60}$ ,  $CO_2@C_{60}$ , and  $CH_3CHO@C_{60}$ , as predicted by G0-MACE-23 and MACE-OFF. The first species has already been discussed in the main text and reported here for comparison. The latter two have not been reported, to the best of our knowledge, in literature and are just a thought experiment for now. Both MLIPs produce energies compatible with DFT, however, MACE-OFF is not able to recover the correct forces for these trajectories, with forces MAE exceeding  $1 \text{ eV } \text{\AA}^{-1}$  in the  $CO_2@C_{60}$  hypothetical species.

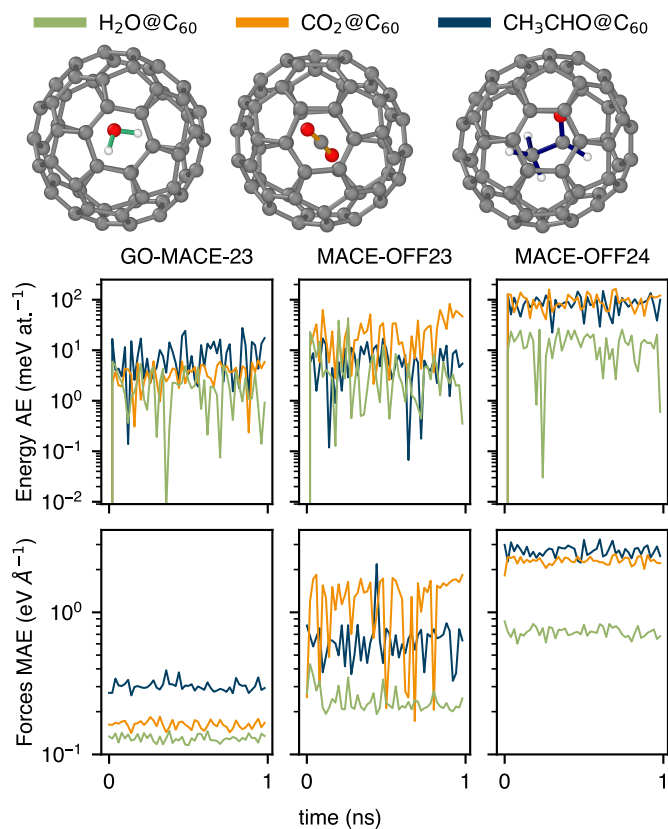

Figure S2: Evolution of energy and forces RMSE, between GO-MACE-23 predictions and the corresponding DFT level of theory (left column) and MACE-OFFs and their corresponding DFT level of theory (centre and right columns), per snapshot of 1 ns trajectories at 500 K of  $\text{H}_2\text{O}$ ,  $\text{CO}_2$ , and  $\text{CH}_3\text{CHO}$  encapsulated in a  $C_{60}$  fullerene. The trajectories are driven by GO-MACE-23.
